# Supplementary material for: A General Approach for Multireference Ground and Excited States using Non-Orthogonal Configuration Interaction
Source: arXiv:1905.02626 ancillary file (2019-05-07)
Supplement: Supplementary file 1 [file HASSupportingInformation.pdf]

# A General Approach for Multireference Ground and Excited States using Non-Orthogonal Configuration Interaction: Supporting Information

Hugh G. A. Burton[1, a)] and Alex J. W. Thom[1]
*Department of Chemistry, Lensfield Road, Cambridge, CB2 1EW, UK*

(Dated: 7 May 2019)

## SI. CYCLOBUTADIENE GEOMETRIES

All coordinates are given in Angstroms.

### A. Rectangular $\mathcal{D}_{2h}$ Geometry:

| | | | |
|---|---|---|---|
| C | -0.6615206 | -0.7841690 | 0.0000000 |
| C | 0.6615206 | -0.7841690 | 0.0000000 |
| C | -0.6615206 | 0.7841690 | 0.0000000 |
| C | 0.6615206 | 0.7841690 | 0.0000000 |
| H | -1.4260054 | -1.5465327 | 0.0000000 |
| H | 1.4260054 | -1.5465327 | 0.0000000 |
| H | -1.4260054 | 1.5465327 | 0.0000000 |
| H | 1.4260054 | 1.5465327 | 0.0000000 |

### B. Square $\mathcal{D}_{4h}$ Geometry:

| | | | |
|---|---|---|---|
| C | -0.6615173 | -0.7840554 | 0.0000000 |
| C | 0.7840554 | -0.6615173 | 0.0000000 |
| C | -0.7840554 | 0.6615173 | 0.0000000 |
| C | 0.6615173 | 0.7840554 | 0.0000000 |
| H | -1.4260274 | -1.5465351 | 0.0000000 |
| H | 1.5465351 | -1.4260274 | 0.0000000 |
| H | -1.5465351 | 1.4260274 | 0.0000000 |
| H | 1.4260274 | 1.5465351 | 0.0000000 |

## SII. SELECTED CONFIGURATION INTERACTION

### A. Computational Details

To obtain an estimate of the exact FCI excitation energies in cyclobutadiene, we iteratively grow the CI expansion using the CIPSI (CI using a perturbative selection made iteratively) approach[1–3] implemented in QUANTUM PACKAGE 2.0.[4] Starting from the CIS wave function, and using the frozen core approximation, the truncated CI space is iteratively grown as large as computationally feasible. At each iteration, we obtain the variational energy $E_{\text{var}}$ of the truncated CI wave function and a second-order pertubative correction $E_{\text{PT2}}$. In the FCI limit we expect $E_{\text{var}} \rightarrow E_{\text{FCI}}$ and $E_{\text{PT2}} \rightarrow 0$. Following previous work,[5–8] we therefore extrapolate $E_{\text{var}}$ against $E_{\text{PT2}}$ to obtain the extrapolated FCI (ex-FCI) estimate $E_{\text{ex-FCI}}$ corresponding to $E_{\text{PT2}} = 0$. Similarly to the approach described by Loos *et al*,[7] we take the average of a two- and three-point linear fit to estimate the value of $E_{\text{ex-FCI}}$, while we use the spread of these fits to assess the error associated with this extrapolation. Using the algorithm implemented in QUANTUM PACKAGE 2.0, the $E_{\text{PT2}}$ correction is evaluated through a hybrid stochastic-deterministic algorithm.[9] To ensure spin-purity and treat ground and excited states as evenly as possible, all the singlet states are determined using a common set of $N_{\text{det}}$ determinants while the triplet state is computed in a separate calculation with a similar number of determinants.

a)Electronic mail: hb407@cam.ac.uk

## B. Results

| $N_{\text{det}}$ | $E_{\text{var}}(^1\text{B}_{1g})$ | $E_{\text{PT2}}(^1\text{B}_{1g})$ | $E_{\text{var}}(^1\text{A}_{1g})$ | $E_{\text{PT2}}(^1\text{A}_{1g})$ | $E_{\text{var}}(^1\text{B}_{2g})$ | $E_{\text{PT2}}(^1\text{B}_{2g})$ |
|---|---|---|---|---|---|---|
| 1241 | −153.60215631 | −0.41582548 | −153.58374982 | −0.36628188 | −153.37352818 | −0.39798242 |
| 2486 | −153.72114173 | −0.40923866 | −153.65884637 | −0.40727047 | −153.64331676 | −0.44311396 |
| 4179 | −153.78292275 | −0.36338945 | −153.72042110 | −0.37272386 | −153.69156830 | −0.38857297 |
| 7598 | −153.84584472 | −0.30630096 | −153.78051331 | −0.31579950 | −153.71998575 | −0.36292551 |
| 14866 | −153.89773366 | −0.26699290 | −153.83163547 | −0.27564084 | −153.77850587 | −0.31269202 |
| 29096 | −153.95957322 | −0.21736905 | −153.89259743 | −0.22559148 | −153.83355773 | −0.26629524 |
| 56974 | −154.01631334 | −0.17291535 | −153.94849719 | −0.17973631 | −153.89698987 | −0.21363023 |
| 110609 | −154.06489067 | −0.13384841 | −153.99626494 | −0.14087948 | −153.95965493 | −0.16126604 |
| 210289 | −154.10123808 | −0.10423209 | −154.03325006 | −0.11072002 | −154.01003710 | −0.11807994 |
| 391967 | −154.12263640 | −0.08659362 | −154.05621615 | −0.09277286 | −154.03838970 | −0.09354860 |
| 705809 | −154.13304090 | −0.07832084 | −154.06969917 | −0.08235484 | −154.04844848 | −0.08503701 |
| 1225595 | −154.13943225 | −0.07338737 | −154.07758731 | −0.07597806 | −154.05363701 | −0.08056273 |
| 2082476 | −154.14468977 | −0.06973087 | −154.08278397 | −0.07171463 | −154.05784823 | −0.07673966 |
| 3609921 | −154.14926746 | −0.06505198 | −154.08737151 | −0.06769769 | −154.06208160 | −0.07347382 |
| 6112945 | −154.15372843 | −0.06174878 | −154.09164123 | −0.06430723 | −154.06614770 | −0.07031188 |
| 10374047 | −154.15827081 | −0.05820367 | −154.09617470 | −0.06087538 | −154.07063171 | −0.06679552 |

TABLE I: Variational energy $E_{\text{var}}$ and perturbative correction $E_{\text{PT2}}$ for the singlet states of square $\mathcal{D}_{4h}$ cyclobutadiene. All energies are given in Hartrees using the cc-pVDZ basis set.

| $N_{\text{det}}$ | $E_{\text{var}}(^3\text{A}_{2g})$ | $E_{\text{PT2}}(^3\text{A}_{2g})$ |
|---|---|---|
| 1241 | −153.66917033 | −0.59769686 |
| 2485 | −153.76478516 | −0.44651819 |
| 4971 | −153.81636535 | −0.38268097 |
| 9947 | −153.87340848 | −0.31894004 |
| 19903 | −153.93385178 | −0.25651560 |
| 39825 | −153.99483965 | −0.19808227 |
| 79655 | −154.05018720 | −0.14733932 |
| 159313 | −154.09350370 | −0.10793298 |
| 318639 | −154.11873101 | −0.08552676 |
| 637337 | −154.13004376 | −0.07657975 |
| 1274669 | −154.13665132 | −0.07131522 |
| 2549261 | −154.14189252 | −0.06685546 |
| 5098453 | −154.14671816 | −0.06251834 |
| 10195851 | −154.15161226 | −0.05850315 |

TABLE II: Variational energy $E_{\text{var}}$ and perturbative correction $E_{\text{PT2}}$ for the triplet ground state of square $\mathcal{D}_{4h}$ cyclobutadiene. All energies are given in Hartrees using the cc-pVDZ basis set.

| | $E_{\text{ex-FCI}}(^1\text{B}_{1g})$ | $E_{\text{ex-FCI}}(^3\text{A}_{2g})$ | $E_{\text{ex-FCI}}(^1\text{A}_{1g})$ | $E_{\text{ex-FCI}}(^1\text{B}_{2g})$ |
|---|---|---|---|---|
| Two-Point | −154.23284756 | −154.22292153 | −154.17659082 | −154.15580827 |
| Three-Point | −154.23480445 | −154.21957696 | −154.17469425 | −154.15614823 |

TABLE III: Extrapolated FCI energy $E_{\text{ex-FCI}}$ for the ground and excited states of square $\mathcal{D}_{4h}$ cyclobutadiene using two- and three-point linear fits. All energies are given in Hartrees using the cc-pVDZ basis set.

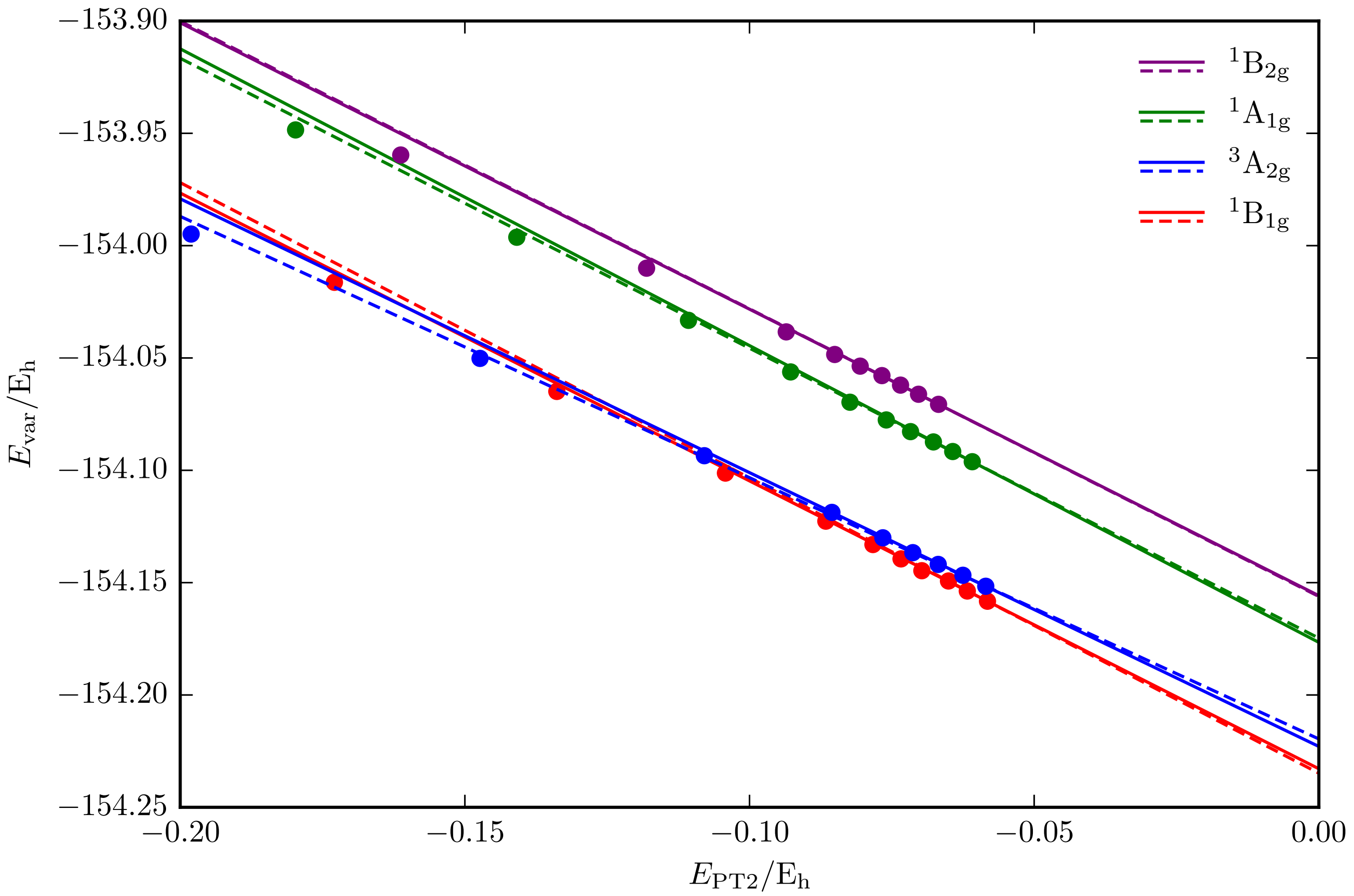


FIG. 1: Extrapolation of the variational energy $E_{var}$ against the perturbative correction $E_{PT2}$ for the ground and excited states of square $\mathcal{D}_{4h}$ cyclobutadiene using two-point (solid lines) and three-point (dashed lines) linear fits.

[1]Evangelisti, S.; Daudey, J. P.; Malrieu, J. P. *Chem. Phys.* **1983**, *75*, 91–102.
[2]Huron, B.; Malrieu, J. P.; Rancurel, P. *J. Chem. Phys.* **1973**, *58*, 5745–5759.
[3]Giner, E.; Scemama, A.; Caffarel, M. *Can. J. Chem.* **2013**, *91*, 879–885.
[4]Garniron, Y. et al. *arXiv:1902.08154* **2019**, Quantum Package 2.0: An Open-Source Determinant-Driven Suite of Programs.
[5]Holmes, A. A.; Umrigar, C. J.; Sharma, S. *J. Chem. Phys.* **2017**, *147*, 164111.
[6]Chien, A. D.; Holmes, A. A.; Otten, M.; Umrigar, C. J.; Sharma, S.; Zimmerman, P. M. *J. Phys. Chem. A* **2018**, *122*, 2714–2722.
[7]Loos, P.-F.; Boggio-Pasqua, M.; Scemama, A.; Caffarel, M.; Jacquemin, D. *J. Chem. Theory Comput.* **2019**, *15*, 1939.
[8]Loos, P.-F.; Scemama, A.; Blondel, A.; Garniron, Y.; Caffarel, M.; Jacquemin, D. *J. Chem. Theory Comput.* **2018**, *14*, 4360–4379.
[9]Garniron, Y.; Scemama, A.; Loos, P.-F.; Caffarel, M. *J. Chem. Phys.* **2017**, *147*, 034101.
